# Supplementary material for: On Demographic Bias in Fingerprint Recognition
Source: arXiv:2205.09318 source file (2022-05-19)
Supplement: Supplementary file 1 [file Supplementary_Material-4.pdf]

# On Demographic Bias in Fingerprint Recognition
## Supplementary Material

### 1. Analyzing outliers in the genuine score distribution for database $D_1$

As discussed in the conclusion of the paper, the demographic differential between black and white subjects observed in Verifinger can be eliminated if the database were to be pruned by removing as few as 13 pairs with the lowest similarity scores out of the 9,112 genuine pairs for white subjects.

There are a total of 47 genuine similarity scores for white subjects that were below the vendor-specified threshold of 48. This document will analyze some of those low similarity scores and discuss the underlying cause. This will help reinforce the conclusion that if the evaluation datasets are free of poor quality or mislabelled images, the demographic bias in a COTS fingerprint recognition system can be either miniscule or eliminated.

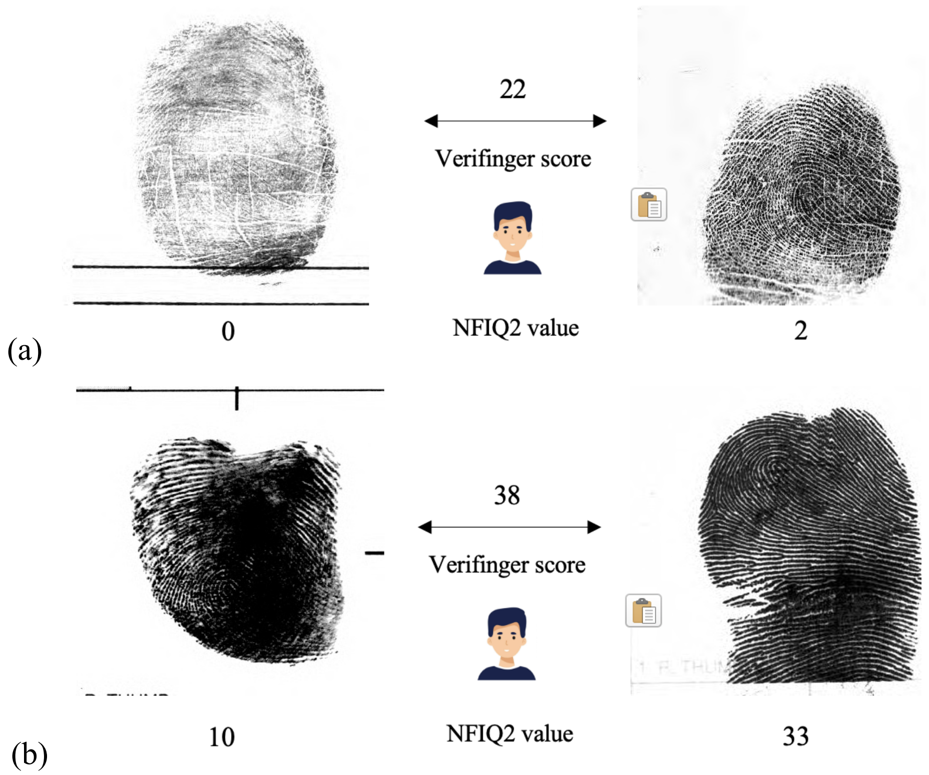

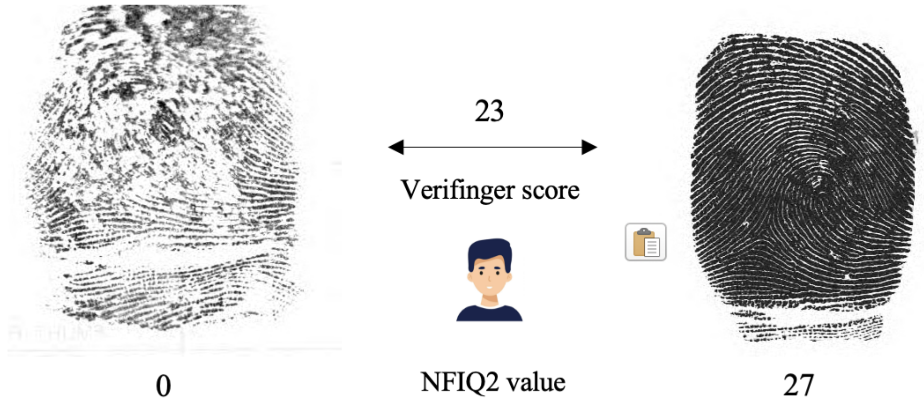
23
Verifinger score
0
NFIQ2 value
27

(c)

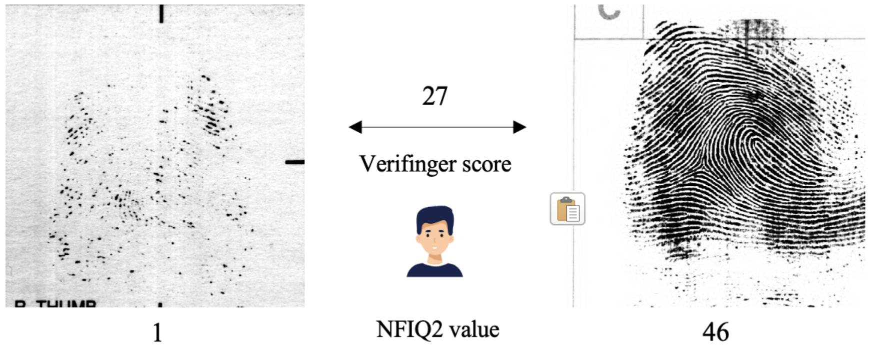
27
Verifinger score
1
NFIQ2 value
46

(d)

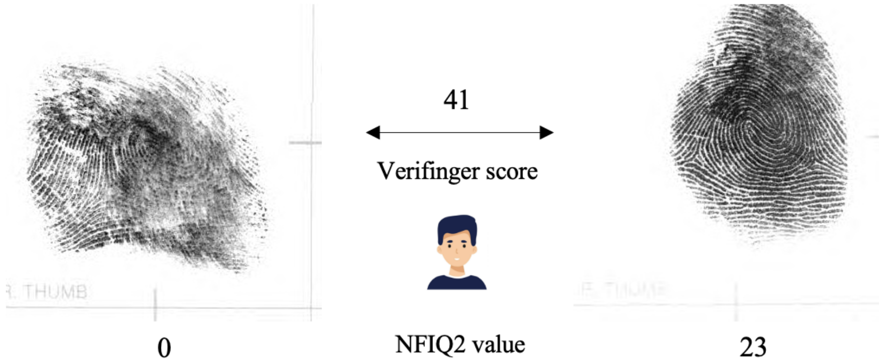
41
Verifinger score
0
NFIQ2 value
23

(e)

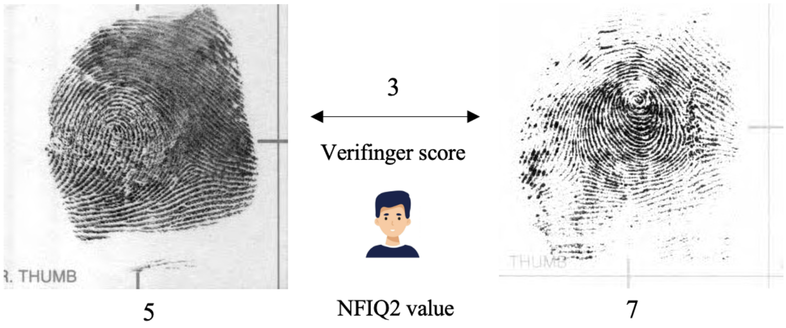
3
Verifinger score
5
NFIQ2 value
7

(f)

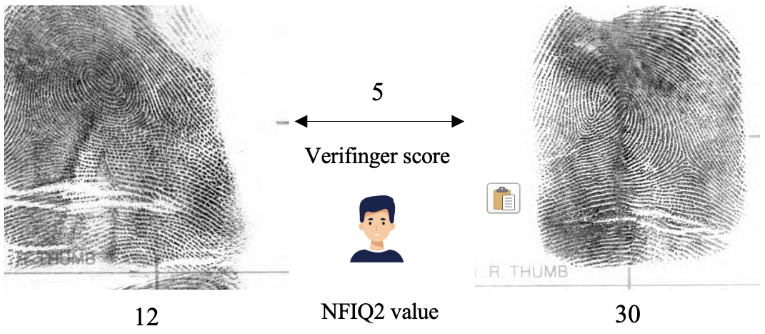
5
Verifinger score
NFIQ2 value
12
30
R. THUMB

(g)

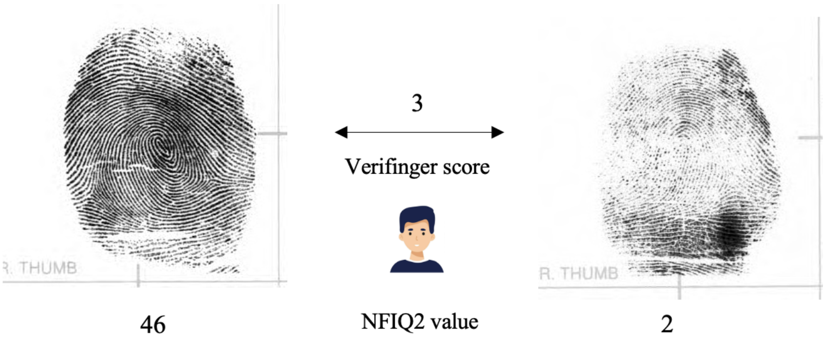
3
Verifinger score
NFIQ2 value
46
2
R. THUMB

(h)

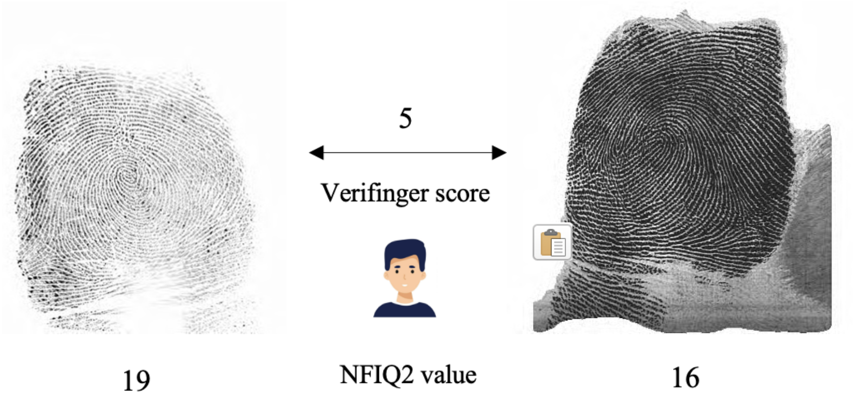
5
Verifinger score
NFIQ2 value
19
16

(i)

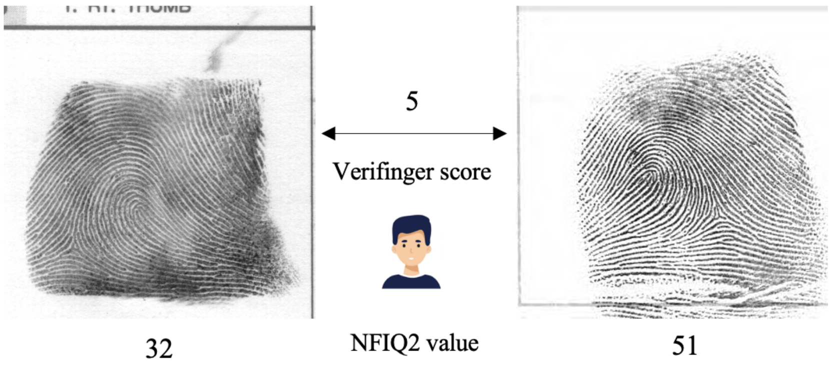
5
Verifinger score
NFIQ2 value
32
51

(j)

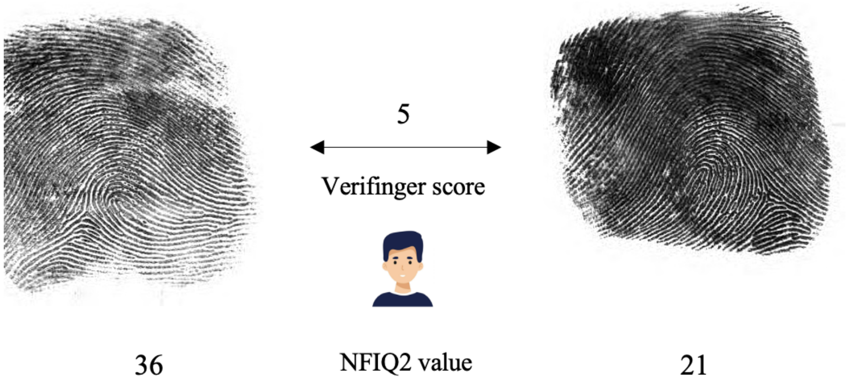


(k)

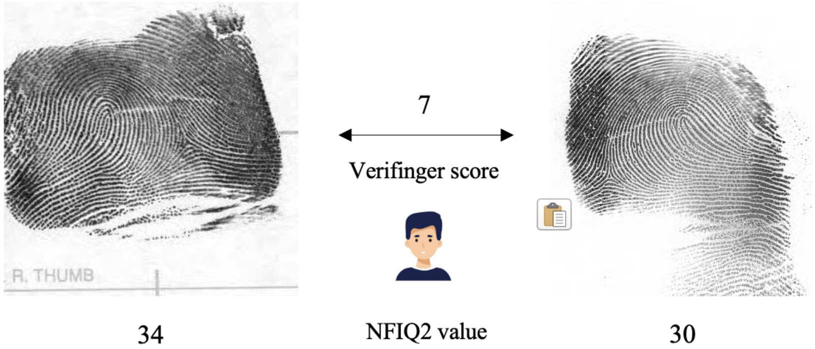


(l)

Figure 1. Thirteen of the lowest genuine similarity scores from Verifinger in dataset $D_1$ . The similarity score for the pair is displayed along with the NFIQ2 value for each fingerprint in the pair. We can see that the low scores are due to either i) low NFIQ2 values or ii) mislabeled fingerprints which cause these scores to be outliers and reduce the matcher performance, in this case for white subjects.

Figure 1 shows examples of genuine pairs whose scores can be considered to be outliers. A majority of these are either low quality or fingerprints that have been incorrectly labeled during data collection. For example, in figure 1 (j), both the fingerprints are labeled as the right thumb of the same subject. However, by visually inspecting the fingerprints, it is evident that they are not from the same finger since the image on the left is a right loop type of fingerprint whereas the image on the right is a left loop. Figures 1 (a) - (e) show images that are correctly labeled but have a low NFIQ2 value and figures 1 (f) - (l) show images that are incorrectly labeled. The low similarity scores skew the TMR of the matcher and provide false evidence of bias. Thus, evaluation databases must be thoroughly inspected for such irregularities before claiming the presence of demographic bias in a biometric recognition system.
